# Supplementary material for: Score Matching Riemannian Diffusion Means
Source: arXiv:2502.13106 source file (2025-02-18)
Supplement: Supplementary file 1 [file societal_impact.tex]

The paper shows how to perform efficient computations on Riemannian manifolds and applicability in a practical settings. The methods shown are general statistical algorithms, and therefore they do not in itself have any negative societal impact. Although, the methods are build on diffusion score matching and can be applied to learned Riemannian manifolds, which has recently been seen to be able to compute high quality deep fakes. Therefore, the methods could potential be used with negative societal impact, even though they in no way are not intended so.
